# Supplementary material for: Bad Students Make Great Teachers: Active Learning Accelerates Large-Scale Visual Understanding
Source: arXiv:2312.05328 source file (2024-10-16)
Supplement: Supplementary file 1 [file X_suppl.tex]

% \clearpage
% \setcounter{page}{1}
% % \maketitlesupplementary

% \appendix

% \section{Appendix: supplementary methods}

% \subsection{Details of total compute calculations}
% \label{app:flops}

% The average FLOPs per learner update for an IID training run is given by:

% $$
% C_{\text{IID}} = 3 F_{\text{learn}}
% $$
% where $F_{\text{learn}}$ is the cost of a single learner inference pass and a gradient update costs $\sim$3$\times$ \ inference passes \cite{jouppi2017datacenter}. The average FLOPs per learner update for easy-reference prioritisation is:

% $$
% C_{\text{easy\_ref}} =
% \big(
% 3 F_{\text{learn}} +
% \rho F_{\text{ref}}
% \big) \beta + 
% 3 F_{\text{ref}}
% $$
% %
% where $\rho = B/b$ (set to $\rho=2.0$ for our experiments) and $\beta$ is the learner speedup vs. IID. The average FLOPs per learner update for RHO is:

% $$
% C_{\text{RHO}} =
% \big(
% 3 F_{\text{learn}} +
% \rho (F_{\text{learn}} + F_{\text{ref}}) 
% \big) \beta + 
% 3 F_{\text{ref}}
% $$
% %
% And for \textit{ActiveCLIP} / \textit{ClassAct}:

% $$
% C_{\text{ClassAct / ActiveCLIP}} =
% \big(
% 3 F_{\text{learn}} +
% 2\rho F_{\text{ref}}
% \big) \beta + 
% 3 F_{\text{ref}}
% $$
% %
% The conditions for compute positivity are therefore:

% $$
% \Big( 3 F_{\text{learn}} + \rho F_{\text{act}} \Big) \beta + 3 F_{\text{ref}}
% < 3 F_{\text{learn}}
% $$
% %
% where $F_{\text{act}}$ is one of $F_{\text{ref}}$, $\big(F_{\text{learn}} + F_{\text{ref}} \big)$ or $2F_{\text{ref}}$ for ``easy reference'', RHO or ClassAct / ActiveCLIP, respectively.

% \subsection{Implementation details: ClassAct}
% \label{app:class}

% \vspace{0.5em} \noindent \textbf{Dataset:} We pretrain on the JFT-300M dataset which contains labels for 18,292 classes collected in a semi-automated fashion. JFT labels are therefore noisy (consistently with other web-scale datasets), with approximately 20\% of the examples being mislabeled. In the ``standard'' setting both reference models and subsequent ClassAct models are trained on the full JFT-300M dataset. 

% \vspace{0.5em} \noindent \textbf{Architectures:} We use standard vision transformers trained with 224\x224 image resolution and a patch size of 16\x16. We consider the standard ViT-Base and ViT-Large variants as learners in our in our main study, and smaller-scale variants (ViT-S and ViT-Tiny) when reducing the scoring-model computation. We introduce even smaller variants to scale down actor computation further, and detail the configurations of this ``ViT-Micro'' family in section \ref{sec:app_small_vits}.

% \vspace{0.5em} \noindent \textbf{Learner Training:} We train visual classifiers with softmax cross-entropy and label smoothing of 0.1. We use the AdamW optimizer \cite{loshchilov2019decoupled} with a cosine learning-rate decay and warmup period of 10k iterations. The maximum learning rate is 0.001 and the weight decay is $10^{-3}$.

% \vspace{0.5em} \noindent \textbf{Evaluation:} We evaluate the performance of the learned model by applying it to a held-out set of JFT images, and measuring top-1 accuracy. Previous work has found that in-domain performance on JFT is highly predictive of out-of-distribution generalization \cite{zhai2022scaling}, hence we leave the study of transfer performance to the multimodal setting (Sec. \ref{app:clip}).

% \subsection{Implementation details: ActiveCLIP}
% \label{app:clip}

% \vspace{0.5em} \noindent \textbf{Datasets:}
% We use paired image-text datasets for contrastive pretraining. We experiment with ALIGN, composed of 1.8B image-text pairs, LTIP, introduced in \cite{alayrac2022flamingo} and consisting of 312M higher-quality images with longer descriptions, and JFT-300M which despite being a classification dataset can be used for contrastive learning by using the labels as the paired text for each image \cite{yu2022coca}.

% \vspace{0.5em} \noindent \textbf{Architectures:} The model consists of a vision and text encoder in the standard contrastive learning setup introduced in \cite{radford2021learning}. We a vision transformer as the visual encoder and a text transformer encoder. We use the Base variant for both the vision and text transformers on the learner, following \cite{dosovitskiy2020image}. The smaller variants used by scoring models are the same as in the classification setup described above. % vary the scale of the vision encoder (Q: how does the text encoder scale?) similar to the image classification setup described above. 

% \vspace{0.5em} \noindent \textbf{Learner Training:} As described in Section \ref{sec:meth-losses} we optimize the model using the standard contrastive loss. We train the entire model with the AdamW optimiser and decay the learning rate using a cosine schedule (following a linear warmup period) with a maximum value of $10^{-3}$. We also use a learnable temperature parameter as described in \cite{radford2021learning} and clip the gradients to a maximum global norm of 1.0. We use a batch size of 16,384 on the learner for each dataset. 

% \vspace{0.5em} \noindent \textbf{Evaluation:}
% We evaluate the model’s zero-shot transfer results on standard multimodal benchmarks---image-text retrieval on COCO \cite{lin2014microsoft} and zero-shot image classification on ImageNet. For COCO, we use the standard technique of comparing image and text representations across the dataset to find the most similar text (or image) for each image (or text). For ImageNet, we precompute the representations for all predefined labels and calculate the most similar label for each image. For zero-shot classification, we also apply the prompt engineering described in \cite{radford2021learning} using the released prompts\footnote{\url{https://github.com/openai/CLIP/blob/main/notebooks/Prompt\_Engineering\_for\_ImageNet.ipynb}}. We average the embeddings for each label across all prompts before calculating similarity with the images. %This gives an improvement of around (add percentage here)


% % TODO

% \subsection{Online ClassAct / ActiveCLIP}

% For our main set of results we implement ClassAct and ActiveCLIP with pretrained reference models, as detailed in Algorithm \ref{alg:classact_algo}. However as detailed in Section \ref{sec:one_pass} ClassAct can also be run in a single training loop, by training the reference model on a super-batch (see Algorithm \ref{alg:classact_online}). 

% % Pretrained RHO algorithm (Class___)
% \begin{algorithm}
% %\algsetup{linenosize=\tiny}
% \small
% \caption{\textit{ClassAct} / \textit{ActiveCLIP}}\label{alg:classact_algo}
% \begin{algorithmic}[1]
% \State \textbf{Input:} Randomly initialized learner model $\theta_l$ and small online model $\theta_o$, small pre-trained reference model $\theta_r$. %Learner and online parameters $(\theta_l, \theta_o)$ uninitialized, reference parameters $\theta_r$ pre-trained. 
% Models use loss $\ell_\textrm{act}$ for scoring data and $\ell_\textrm{learn}$ for computing updates. Dataset $\mathcal{D}$, batch size $B$, sub-batch size $b<B$.
% \While{training}
%     \State $X \sim \mathcal{D}$, where $|X| = B$ \Comment{Sample IID}
%     \State $S = \ell_{\text{act}}(X | \theta_o) - \ell_{\text{act}}(X | \theta_r)$ \Comment{Get scores}
%     \State $I \sim \text{SoftMax}(S)$, where $|I| = b$ \Comment{Sample indices}
%     \State $Y = X[I]$ \Comment{Collect sub-batch}
%     % \State $Y \sim \text{SoftMax}(X|S)$, where $|Y| = b$ \Comment{Sample sub-batch}
%     \State $\theta_l \leftarrow \text{Adam}[\nabla_{\theta_l} \ell_{\text{learn}}(Y|\theta_l)]$ \Comment{Update learner model}
%     \State $\theta_o \leftarrow \text{Adam}[\nabla_{\theta_o} \ell_{\text{learn}}(Y|\theta_o)]$ \Comment{Update online model}
% \EndWhile
% \end{algorithmic}

% \end{algorithm}


% % One-pass RHO algorithm (Class___)
% \begin{algorithm}
% %\algsetup{linenosize=\tiny}
% \small
% \caption{Online ClassAct / ActiveCLIP}
% \begin{algorithmic}[1]
% \State \textbf{Input:} Randomly initialized learner model $\theta_l$, small online and reference models $\theta_o$ and $\theta_r$. Models use loss $\ell_\textrm{act}$ for scoring data and $\ell_\textrm{learn}$ for computing updates. Dataset $\mathcal{D}$, batch size $B$, sub-batch size $b<B$. Fast and slow learning rates $\alpha$ and $\beta$.
% \While{training}
%     \State $X \sim \mathcal{D}$, where $|X| = B$ \Comment{Sample IID}
%     \State $S = \ell_{\text{act}}(X; \theta_o) - \ell_{\text{act}}(X; \theta_r)$ \Comment{Get scores}
%     \State $\theta_r \leftarrow \text{Adam}_{\alpha}[\nabla_{\theta_r} \ell_{\text{learn}}(X|\theta_l)]$ \Comment{Update ref. model}
%     \State $I \sim \text{SoftMax}(S)$, where $|I| = b$ \Comment{Sample indices}
%     \State $Y = X[I]$ \Comment{Collect sub-batch}
%     % \State $Y \sim \text{SoftMax}(X|S)$, where $|Y| = b$ \Comment{Sample sub-batch}
%     \State $\theta_l \leftarrow \text{Adam}_{\beta}[\nabla_{\theta_l} \ell_{\text{learn}}(Y|\theta_l)]$ \Comment{Update learner model}
%     \State $\theta_o \leftarrow \text{Adam}_{\beta}[\nabla_{\theta_o} \ell_{\text{learn}}(Y|\theta_o)]$ \Comment{Update online model}
% \EndWhile
% \end{algorithmic}
% \label{alg:classact_online}
% \end{algorithm}

% We found that $B=10b$ was sufficient to reproduce the pre-trained reference (Algorithm \ref{alg:classact_online}) case where $B=2b$, as described Section \ref{sec:one_pass}. It is possible that the super-batch size could be shrunk, but we did not evaluate our method in between these values.

% % Python code is less readable IMO
% \iffalse
% \begin{minted}[frame=lines, framesep=2mm, baselinestretch=1.2, fontsize=\tiny, linenos]{python}

% # Imports
% from jax.numpy import exp
% from jax import grad, random
% from optimizer import update

% # Initialise 
% B, b # Big and small batch sizes
% lossfn_big, lossfn_small # Big and small model loss functions
% θ_learner # Big model parameters
% Φ_online, Φ_ref # Two sets of small model parameters

% # Training loop
% while training:
%     big_batch = sample_iid(batch_size=B)
%     losses_online = lossfn_small(Φ_online, big_batch)
%     losses_ref = lossfn_ref(Φ_ref, big_batch)
%     scores = exp(losses_online - losses_ref)
%     grads_ref = grad(lossfn_ref, 0)(Φ_ref, big_batch)
%     Φ_ref = update(Φ_ref, grads_ref)
%     small_batch = random.choice(a=big_batch, p=scores, sample_shape=(b,))
%     grads_online = grad(lossfn_online, 0)(Φ_online, small_batch)
%     Φ_online = update(Φ_online, grads_online)
%     grads_learne = grad(lossfn_learner, 0)(Φ_learner, small_batch)
%     Φ_learner = update(Φ_learner, grads_learner)
% assert b <= B

% while training:
%     big_batch = sample_iid(batch_size=B)
    
% \end{minted}\fi

% \subsection{Analyzing learnability scores}

% Here we examine learnability scores in the case of small differences between the online and reference models $\theta^t, \theta^*$. In this case, we can apply a Taylor expansion of the reference-model loss: 
% \begin{equation}
%     \ell(\vx_i | \theta^*) \approx  \ell(\vx_i | \theta^t) + (\theta^* - \theta^t) \cdot \nabla_{\theta} \ell( \vx_i |\theta^t)
% \end{equation}
% and learnability scores simplify to the alignment between the gradient of the loss with respect to the online parameters, and the difference between online and reference parameters:
% \begin{align}
% \label{eq:learn_analysis}
% s^\textrm{learn}(\vx_i | \theta^t, \theta^*)
% & =  \ell(\vx_i | \theta^t) - \ell(\vx_i | \theta^*) \\ 
% & \approx  (\theta^t - \theta^*) \cdot \nabla_{\theta} \ell( \vx_i |\theta^t).
% \end{align}
% This yields a simple explanation for the relevance of learnability scores: data points whose gradient aligns well with the ``direction of travel'' (\ie the difference between the current model state and the fully-trained one) will be prioritized. We can further simplify this expression in the case where the reference model is the result of a single, global update with respect to gradients from a batch of data $\{\vx_j\}$:
% \begin{align}
%     \theta^* & = \theta^t - \lambda \nabla_{\theta} \ell( \{ \vx_j \} |\theta) \\ 
%     s^\textrm{learn}(\vx_i | \theta^t, \theta^*) & \approx \lambda \nabla_{\theta} \ell( \vx_i |\theta^t) \cdot \nabla_{\theta} \ell( \{\vx_j\} | \theta^t)
% \end{align}
% In this case, an example's learnability reduces to the alignment of its gradient to those of the batch. In particular, these scores de-prioritize examples which are trivially solved (small gradients) or noisy (mis-aligned with the batch gradient). 

% Finally, we note that learnability scores reduce to gradient-norm prioritization \cite{paul2021deep} if we make the further (more stringent) assumption that the reference model is the result of a single update with respect to \textit{this example's gradient only}:
% \begin{align}
%     \theta^* & = \theta^t - \lambda \nabla_{\theta} \ell( \vx_i |\theta) \\ 
%     s^\textrm{learn}(\vx_i | \theta^t, \theta^*) & \approx s^\textrm{grad}(\vx_i | \theta^t) =  \lambda \left|\left| \nabla_{\theta} \ell( \vx_i |\theta^t) \right|\right|^2
% \end{align}
% While this prioritization effectively discards examples with small gradients, it does not benefit from the denoising properties of the more general formulation of learnability, as noisy examples can exhibit large gradients. 

% \subsection{Learning infrastructure}

% Our learning infrastructure Figure \ref{fig:learning_infra} draws inspiration from distributed reinforcement learning (DRL) \cite{espeholt2018impala}. In contrast to DRL, where run loops generate data through interactions with an environment, run loops in our system are modified to read offline data. In addition to obtaining data, run loops run inference on the data via remote inference servers and write the inference outputs to prioritized replay data stores \cite{cassirer2021reverb}. The distributed nodes of our learning setup are configured and connected using \cite{yang2021launchpad}.

% Data stored is sampled from the prioritized replay based on priorities determined during inference. Remote inference servers continuously run inference at specific batch sizes, in parallel to learning. Parameters of the inference servers are updated after each learning step.

% \begin{figure}[t]
%   \centering
%   \includegraphics[scale=0.38]{figures/infra.png}
%   \caption{The main nodes of our distributed learning infrastructure are: (1) a learner that continuously updates model parameters based on sampled data, (2) an inference server which computes priorities of uniformly sampled data, and (3) a prioritized replay which receives data and priorities from the inference server and samples prioritized data for learning. The critical aspect of our system is adaptive data prioritization which is enabled by keeping inference parameters in sync with the learner. We employ separate prioritized replay and inference server nodes per dataset. We also employ run loop nodes (not shown in the diagram) for reading and writing data. Run loop nodes can run as threads on the inference server node or remotely, to prevent extra load on inference servers.}
%   \label{fig:learning_infra}
% \end{figure}

% For stability, we control the ratio of data sampled to data inserted in all of our experiments. For example, a samples-per-insert (SPI) ratio of 0.5 means that half of the inserted data does not get sampled, ensuring the learner focuses on the most relevant data. Each data item is sampled at most once. These two constraints impose minimum inference requirements to fully saturate the learner, which we separately tune for each experiment by scaling up the topology of the inference server.

% Our infrastructure is designed to work with multiple datasets. In this case, we use separate remote inference server, run loops, and prioritized replay for each dataset, and set the batch size per dataset.

% To continuously assess the performance of our models, we add data evaluator nodes which measure performance on held-out datasets while periodically pulling the latest parameters from the learner node.



% %  All models use ViT-B/16 encoders, with 224\x224 image resolution, except SigLIP which uses 256\x256.

% \subsection{Small ViT models} \label{sec:app_small_vits}

% We extended the suite of ViT models presented in \cite{zhai2022scaling} by further scaling down the ViT-Ti model as shown in Table \ref{tab:small_vits}.

% \begin{table}[t]
% \footnotesize
% \centering
% \begin{tabular}{ccccccc}
% Name     & Width & Depth & MLP  & Heads & Mio- & GFLOPs \\
%      &  &  &   &  & -Params & $224^2$ \\
% \hline
% L        & 1024  & 24    & 4096 & 16    & 304        & 61.6           \\
% B        & 768   & 12    & 3072 & 12    & 86         & 17.6           \\
% S        & 384   & 12    & 3072 & 12    & 22         & 4.6            \\
% Ti       & 192   & 12    & 768  & 3     & 5.6        & 1.3            \\
% Mu\_6-3  & 192   & 6     & 768  & 3     & 2.8        & 1.24           \\
% Mu\_12-2 & 128   & 12    & 512  & 2     & 2.5        & 1.23           \\
% Mu\_6-2  & 128   & 6     & 512  & 2     & 0.66       & 0.48           \\
% Mu\_12-1 & 64    & 12    & 256  & 1     & 1.3        & 0.23           \\
% Mu\_6-1  & 64    & 6     & 256  & 1     & 0.36       & 0.203           \\
% Mu\_3-1  & 64    & 3     & 256  & 1     & 0.22       & 0.065           \\
% Mu\_2-1  & 64    & 2     & 256  & 1     & 0.16       & 0.033           \\
% Mu\_1-1  & 64    & 1     & 256  & 1     & 0.12       & 0.011  
% \end{tabular}
% \caption{\textbf{ViT model details}. Configurations, parameter counts, and FLOPs associated with small ViT models.}
% \label{tab:small_vits}
% \end{table}
